# Supplementary material for: LightDepth: Single-View Depth Self-Supervision from Illumination Decline
Source: arXiv:2308.10525 source file (2023-09-20)
Supplement: Supplementary file 1 [file suplementary.tex]

\setcounter{figure}{0}
\setcounter{section}{0}
\section{Network architectures}
\textbf{LightDepth U-Net}
We use a U-Net architecture with skip connections and two decoders. Our encoder is a ResNet18\cite{He2015} initialized with the weights from ImageNet\cite{deng2009imagenet}. Regarding the decoders, our albedo decoder uses sigmoid activation function and our depth decoder ELU+1 activation function after the last convolution. 

\textbf{LightDepth DPT}
We extend LightDepth DPT \cite{Ranftl_2021_ICCV} adding a branch for the prediction of albedo decoder. For the depth estimation, we initialize the encoder and depth decoder with DPT Hybrid weights. For albedo estimation, we train the albedo decoder from scratch. In our pipeline, we use the half of resolution than the original images for training, upsampling the outputs with bilinear interpolation.

\begin{figure}[b!]
\centering
  \includegraphics[width=0.5\linewidth]{images/albedo head.pdf}
\caption{Albedo estimation head}
\label{fig:head}
\end{figure}
Figure \ref{fig:head} presents the head for the albedo decoder that includes an Sigmoid activation function.

\section{Datasets}
Table \ref{tab:c3vdsplit} shows which sections of the C3VD were used for training / testing. 
We split into sections to ensure a fair comparison along the dataset. Regarding real endoscopy images, we use with the sequence 051, 009 and 058 of the EndoMapper dataset. 

\begin{table}[h!]
    \resizebox{\linewidth}{!}{
\begin{tabular}{|c|c|c|c|c|}
\hline Model  & Texture & Video  & Frames & Stage   \\ \hline
Cecum & 1 & b&765& Train  \\
Cecum & 2 & b&1120& Train  \\
Cecum & 2 & c&595& Train  \\
Cecum & 4 & a&465&   Train\\
Cecum &4 & b&425& Train  \\

Sigmoid Colon &1 & a&800& Train  \\
Sigmoid Colon &2 & a&513& Train  \\
Sigmoid Colon &3 & b&536& Train  \\
Transcending Colon &1 & a&61& Train  \\
Transcending Colon &1 & b&700& Train  \\
Transcending Colon &2 & b&102& Train  \\
Transcending Colon &4 & b&595& Train  \\
Descending Colon &4 & a&74& Train  \\

\hline
Cecum & 1 & a&275& Test  \\
Cecum & 2 & a&370& Test  \\
Cecum & 3 & a&730& Test  \\
Descending Colon &4 & a&74& Test  \\
Sigmoid Colon &3 & a&610& Test  \\
Transcending Colon &2 & a&194& Test  \\
Transcending Colon &3 & a&250& Test  \\
Transcending Colon &4 & a&382& Test  \\
\hline
    \end{tabular}
    }
    \label{tab:c3vdsplit}
    \caption{Dataset Split for C3VD }
\end{table}

\section{Normals from Depth}
Figure \ref{fig:normals} shows examples of Open3d\cite{Zhou2018Open3D}, in-house, U-Net and TFtN\cite{fan2021three} used in the analysis.

\begin{figure}[h!]
  \includegraphics[width=\linewidth]{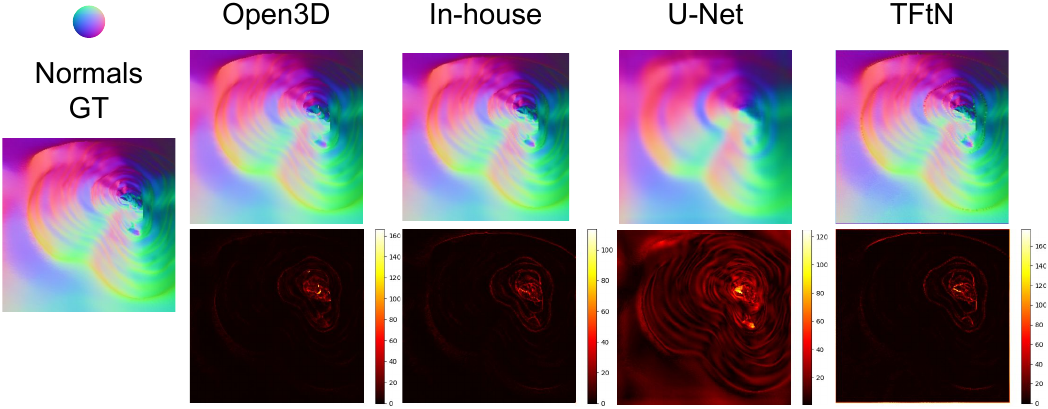}
\caption{Quantitative results of different approaches to obtaining surface normals from a depth map.}
\label{fig:normals}
\end{figure}

\section{Additional results}
We present additional quantitative and qualitative results. Figure \ref{fig:additionalreal} shows additional qualitative results of LightDepthDPT TTR in real colonoscopy and gastroscopy procedures. Figure \ref{fig:additionalphantom} shows quantitative results of LightDepth U-Net in the transverse and cecum sections of the C3VD.

Finally, in Figure \ref{fig:additionalsynth} we show examples of LightDepth U-Net in our in-house synthetic dataset. The predicted depth and normals capture the shape of the colon sections, as shown in the 3D reconstruction. The albedo map appears brighter as we fix Value Channel to $V = 100$. Our method recovers the different albedo of mucosa and blood vessels.

\begin{figure*}
  \includegraphics[width=\textwidth]{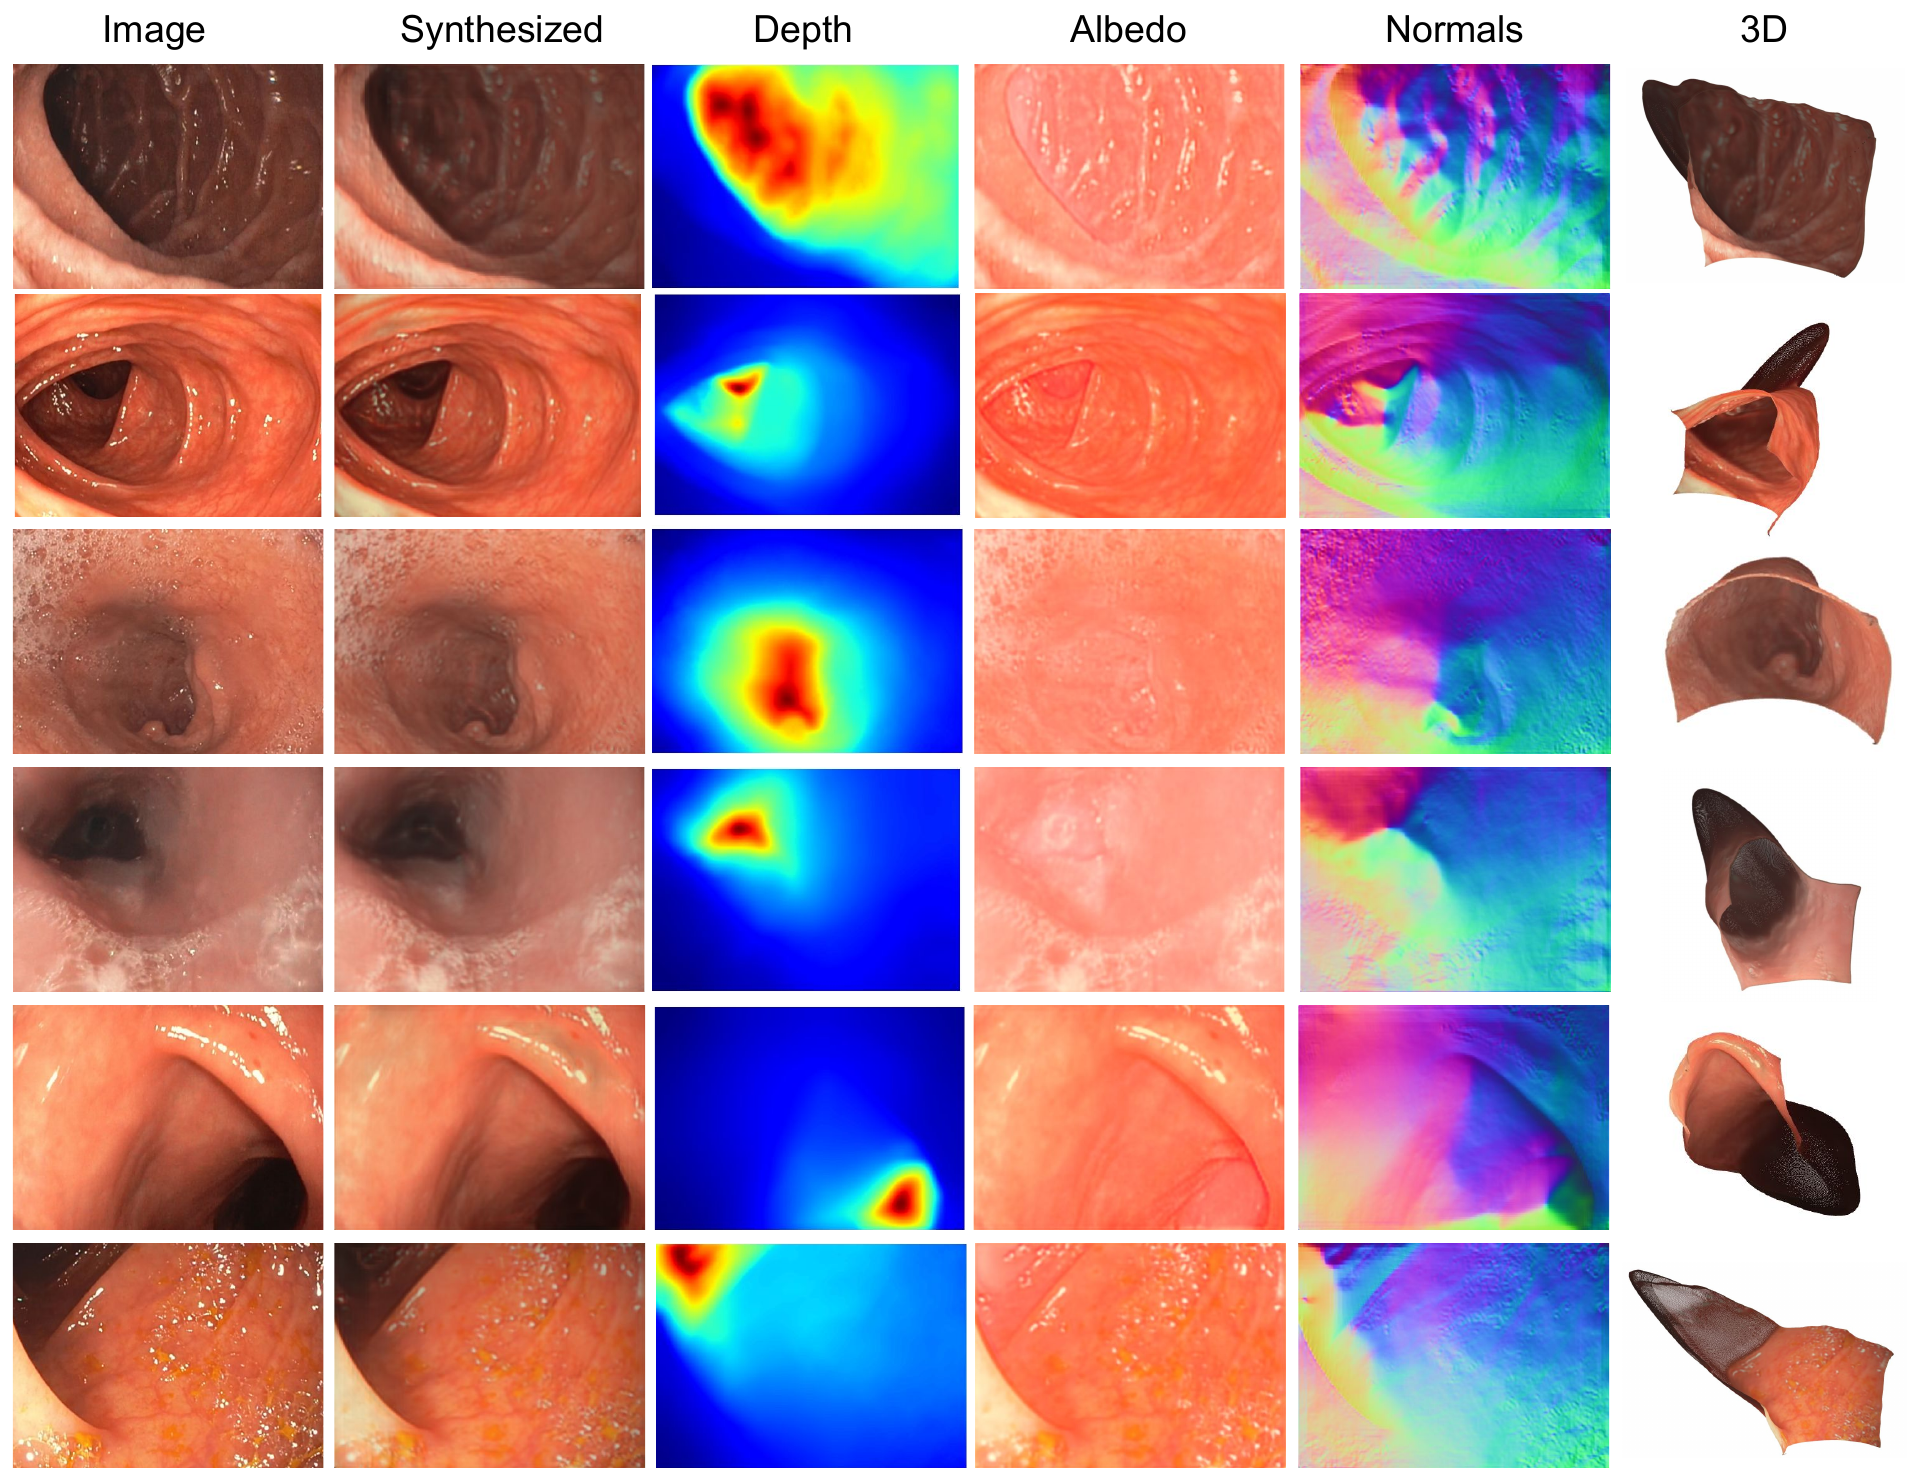}
\caption{Additional qualitative examples of LightDepthDPT in real colonoscopy and gastroscopy procedures.}
\label{fig:additionalreal}
\end{figure*}

\begin{figure*}
  \includegraphics[width=\textwidth]{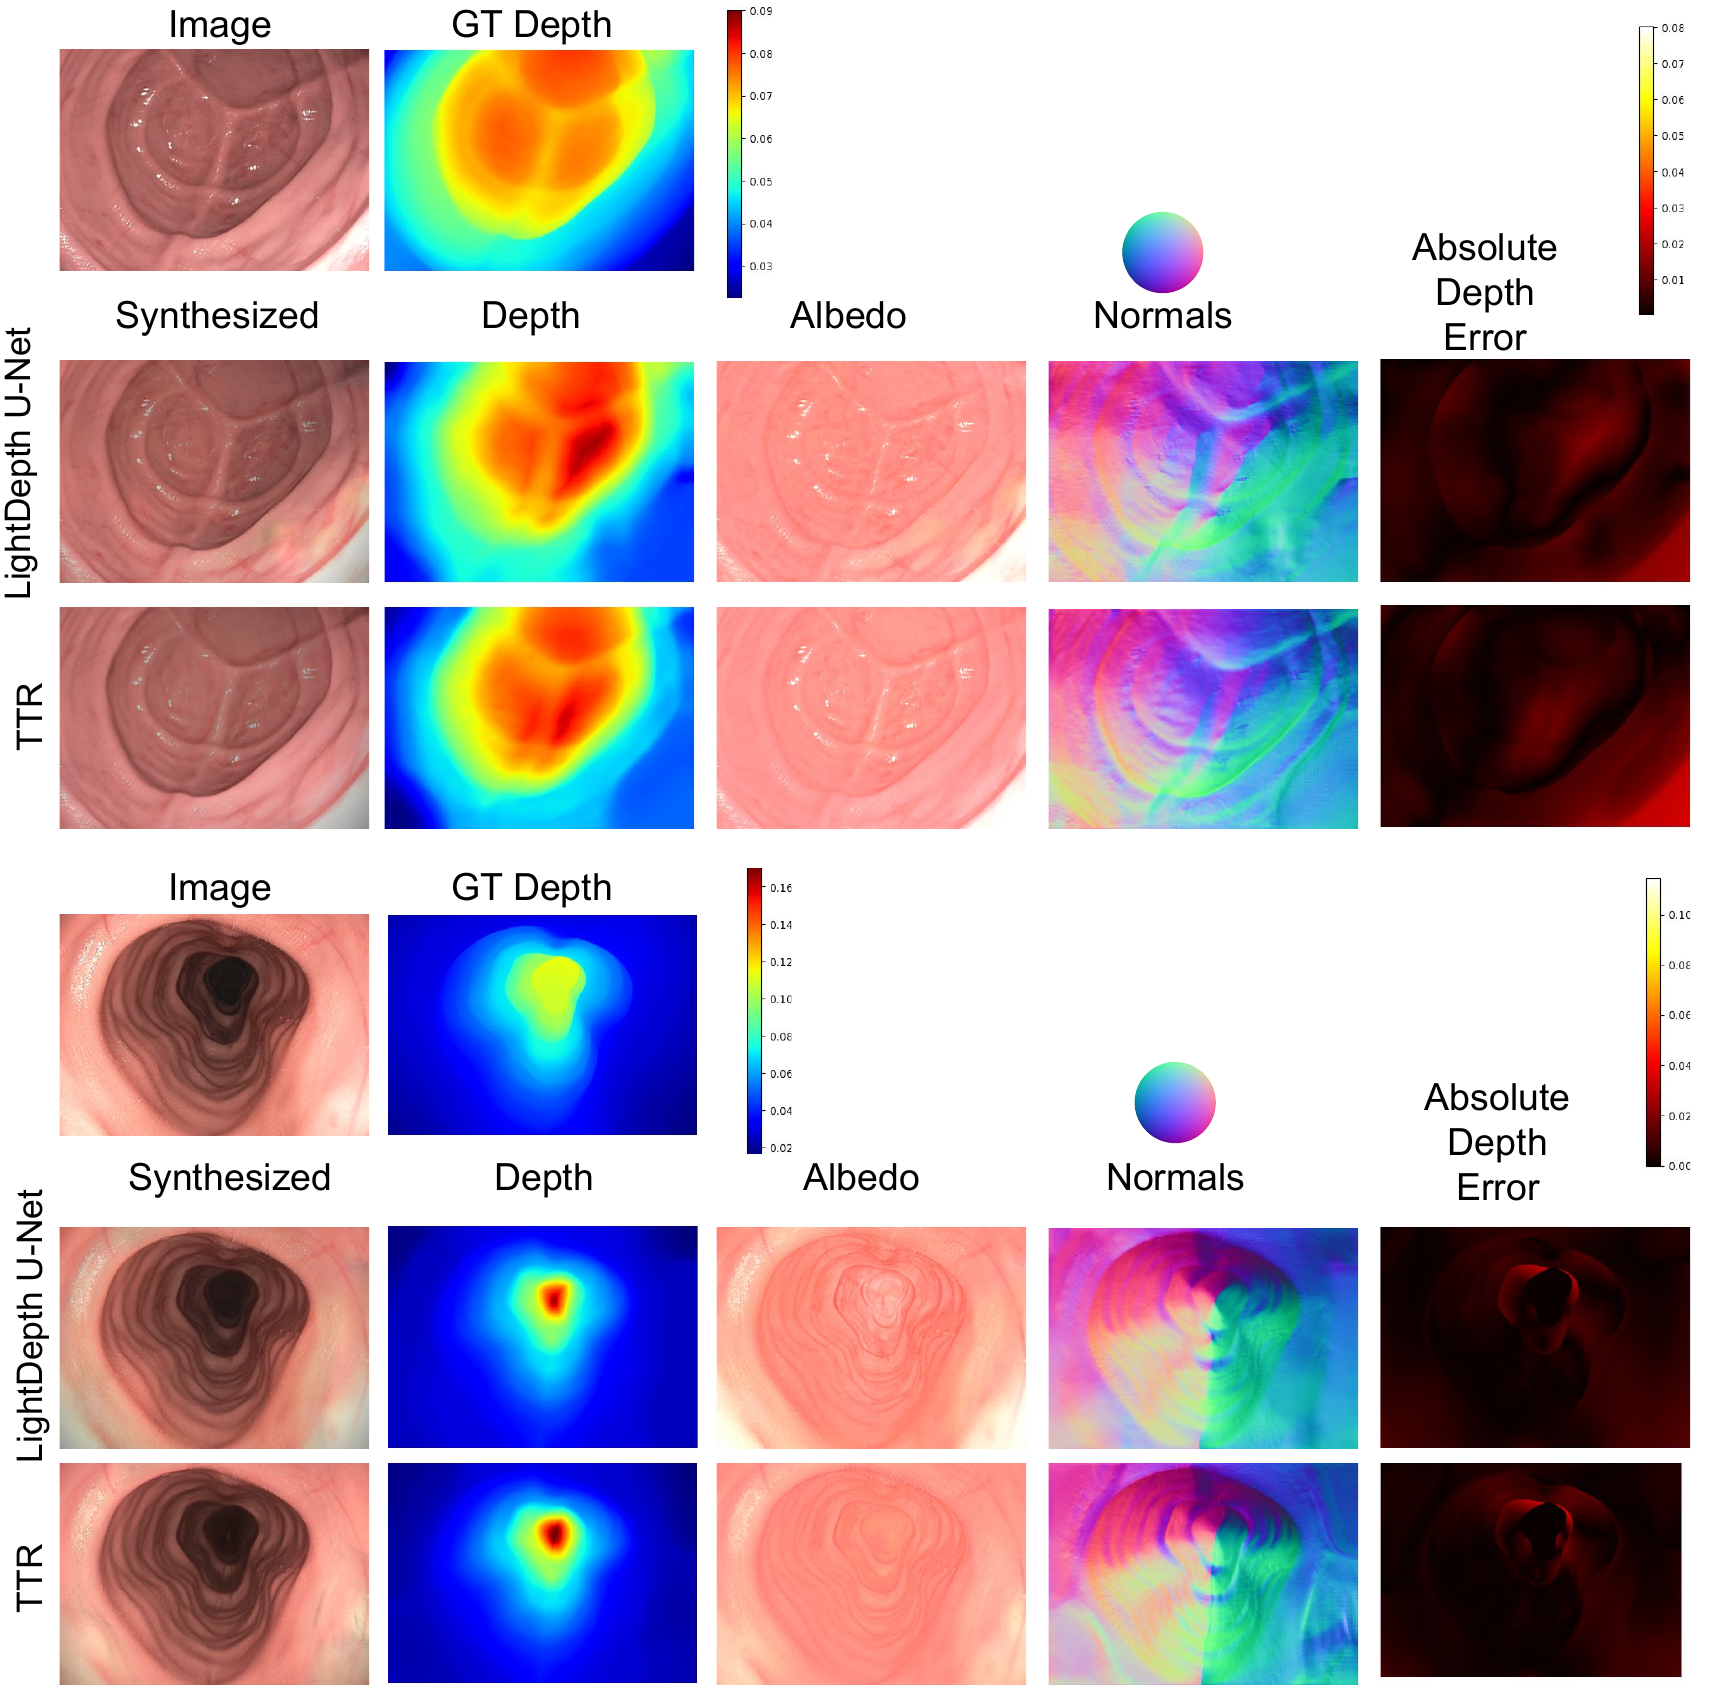}
\caption{Additional quantitative examples of LightDepth U-Net in C3VD.}
\label{fig:additionalphantom}
\end{figure*}
% https://docs.google.com/drawings/d/1lfrF9Dh3P6d6aXvm4xdQp0LtqSJL-fxGNjDeit0l3eM/edit?usp=share_link
% Images 71 and 290 of synthetic dataset
\begin{figure*}
  \includegraphics[width=\textwidth]{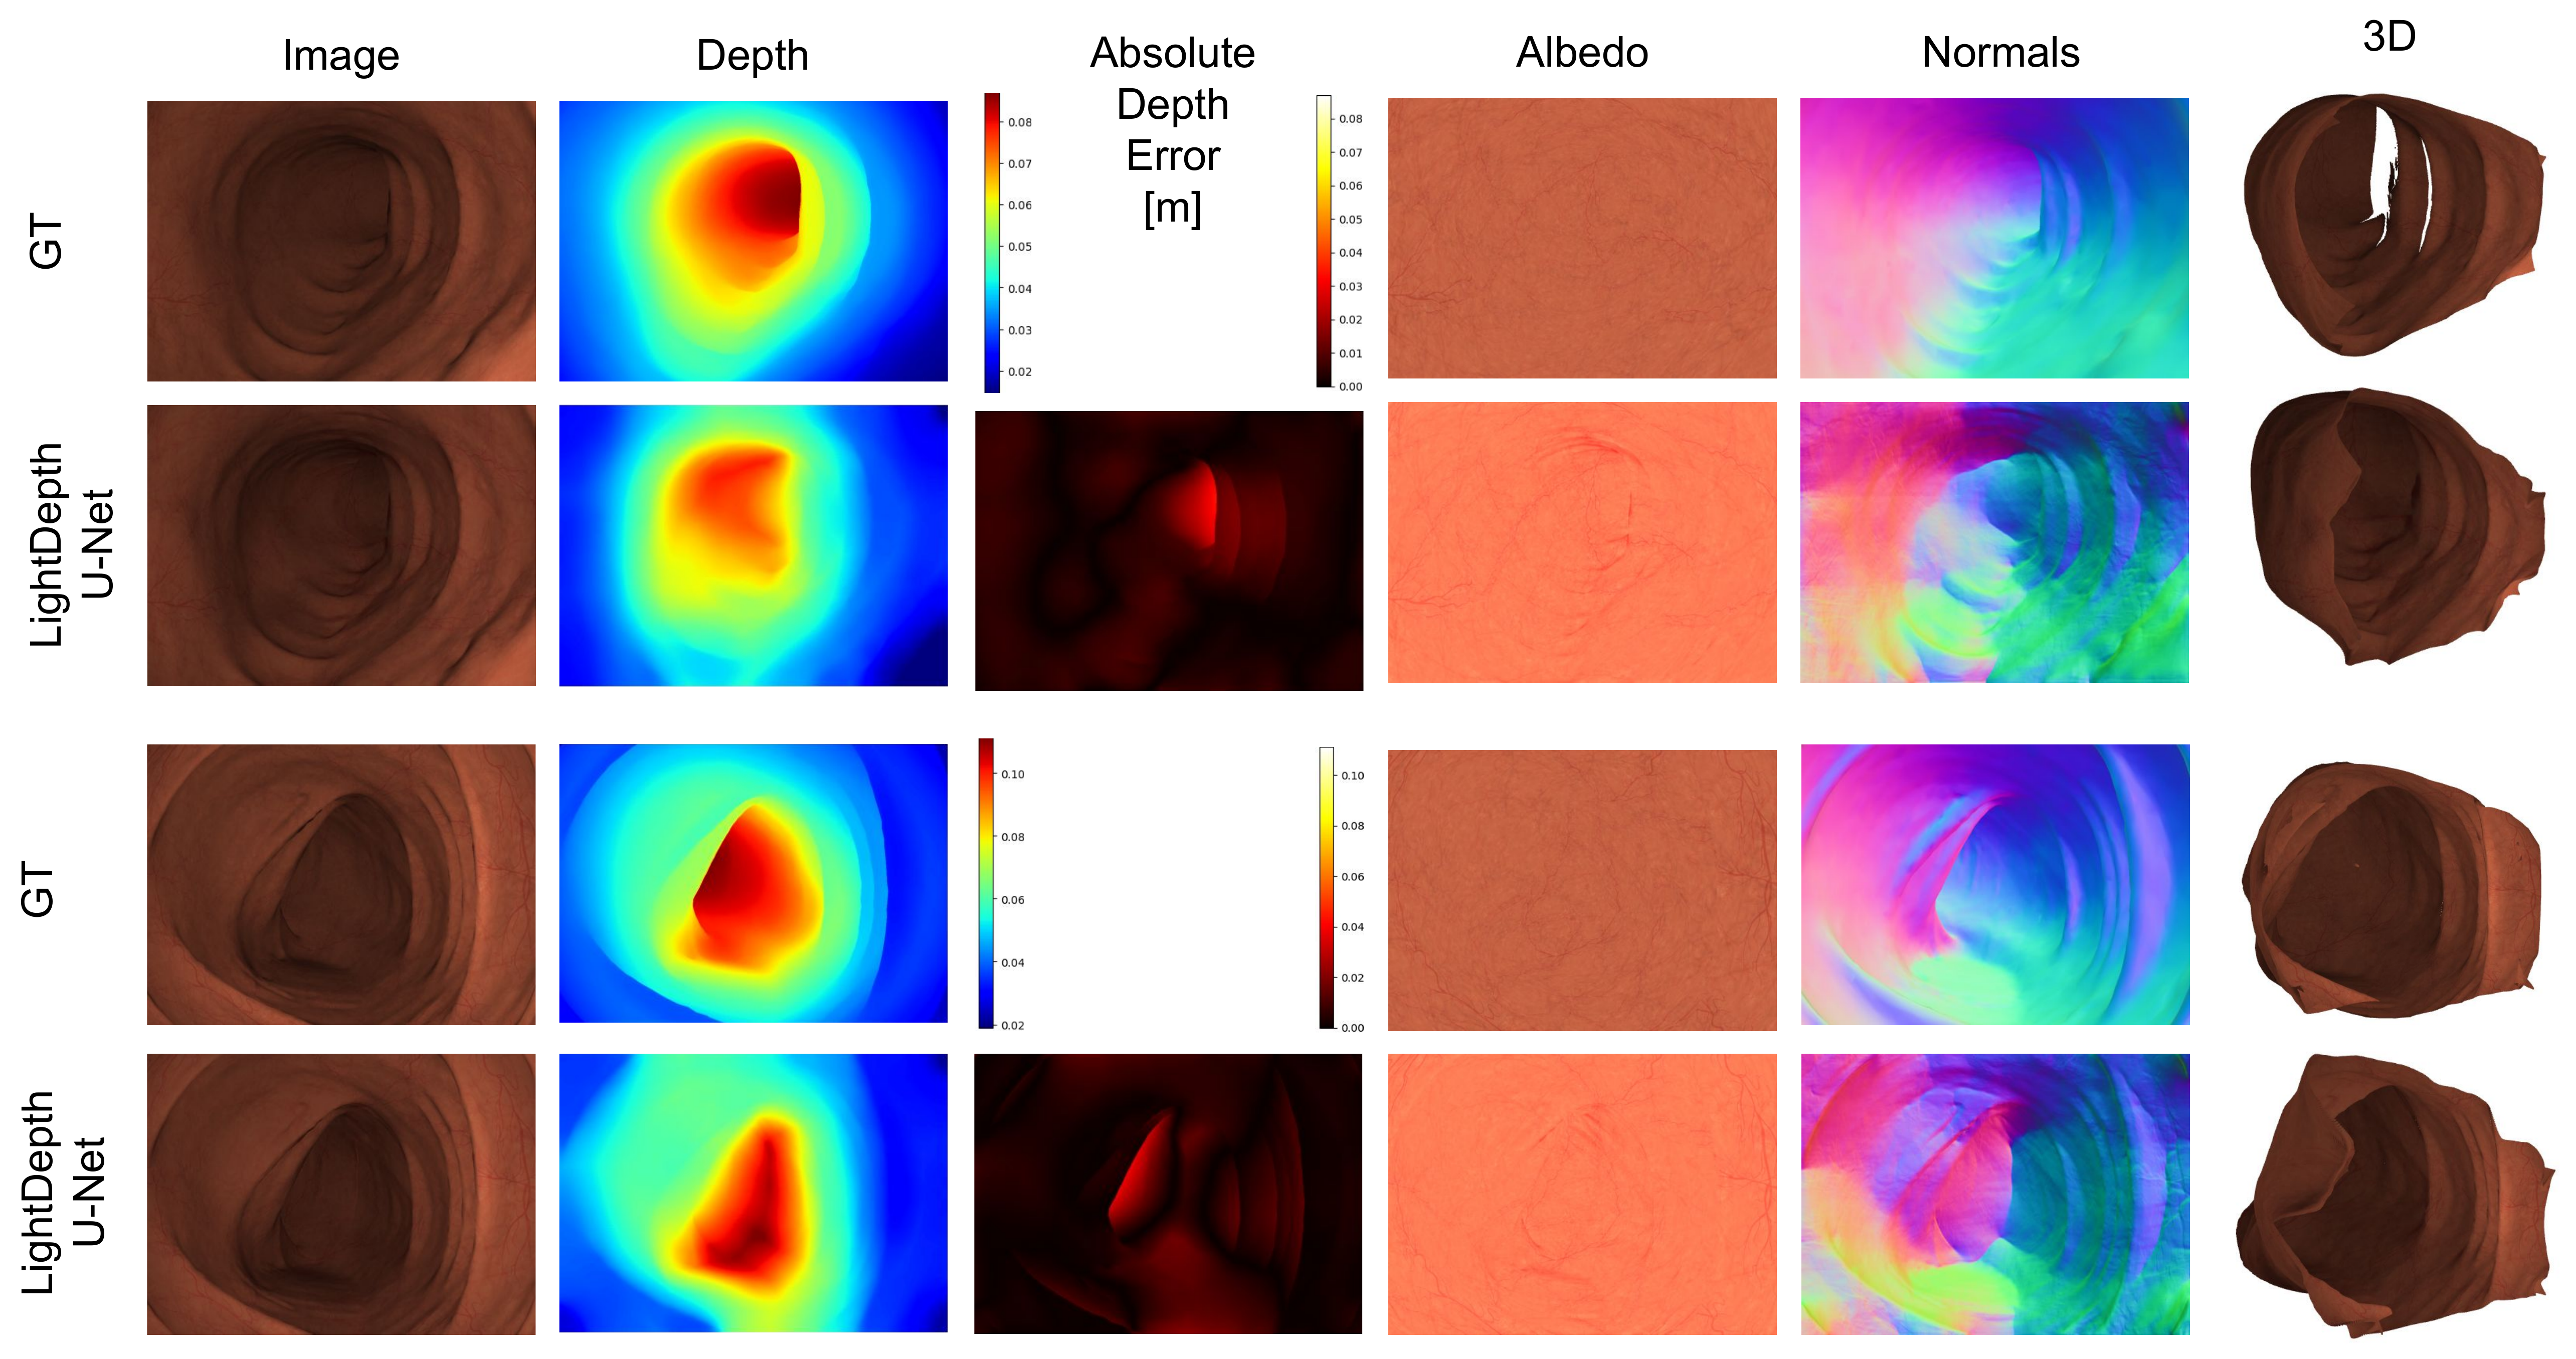}
\caption{Qualitative examples of LightDepth in Synthetic dataset.}
\label{fig:additionalsynth}
\end{figure*}
